# Supplementary material for: Signatures of motor susceptibility in the dynamics of a tracer particle in an active gel
Source: arXiv:1806.08921 ancillary file (2018-06-23)
Supplement: Supplementary file 1 [file SI.pdf]

# Signatures of motor susceptibility in the dynamics of a tracer particle in an active gel

## Supplemental Material

Nitzan Razin,<sup>1</sup> Raphael Voituriez,<sup>2</sup> and Nir S. Gov<sup>1</sup>

<sup>1</sup>*Department of Chemical and Biological Physics,  
Weizmann Institute of Science, Rehovot 76100, Israel*

<sup>2</sup>*Laboratoire Jean Perrin and Laboratoire de Physique Théorique de la Matière Condensée,  
CNRS/Université Pierre et Marie Curie, 75005 Paris, France*

(Dated: June 21, 2018)

### 1. EXPONENTIAL TAIL OF THE VAN HOVE DISTRIBUTION IN THE WEAK CONFINEMENT LIMIT

We prove below that in the limit of negligible bulk elasticity  $k = 0$ , the van Hove distribution for a particle pushed by adamant motors has exponential tails. We neglect thermal fluctuations and other white noise forces - and thus assume that the particle moves freely due to the motor forces only. Since  $k = 0$ , the particle displacement is a sum of independent contributions due to each of the motors. We assume in the calculation of the van Hove distribution below that there is one motor ( $N = 1$ ), and the result for a general  $N$  can be obtained from the distribution for  $N = 1$  by  $P(\Delta x(\Delta t); N) = P(\Delta x(N\Delta t); N = 1)$ .

We will call the displacement due to a single motor on duration a single step, and denote the displacement due to the  $i$ -th step  $x_i$ . The total displacement of the particle within a time  $\Delta t$  can thus be written as:

$$\Delta x = x_0 + \sum_{i=1}^n x_i + x_{n+1} \quad (S1)$$

where  $x_i$  for  $i = 1, \dots, n$  are all steps as defined above, and  $x_0$  and  $x_{n+1}$  are the displacement caused by possible incomplete steps that begin at the beginning of  $\Delta t$  or end when it ends, and not due to a motor state change. We shall assume that  $\Delta t$  is large enough with respect to the average on time  $k_{\text{off}}^{-1}$  so that the contribution to  $\Delta x$  from incomplete steps is negligible:  $\sum_{i=1}^n x_i \gg x_0, x_{n+1}$  (note that this assumption is consistent with the fact that we are interested in the tail of  $P(\Delta x(\Delta t))$ ).

Using the law of total probability, the van Hove distribution can be written as:

$$P(\Delta x(\Delta t)) = \sum_{n=0}^{\infty} P(\Delta x(\Delta t)|n(\Delta t)) P_n(n(\Delta t)) \quad (S2)$$

where  $P_n(n(\Delta t))$  is the distribution of the number of steps  $n$  that occurred within  $\Delta t$ . We will now calculate  $P(\Delta x(\Delta t)|n(\Delta t))$ , the distribution of the displacement  $\Delta x \approx \sum_{i=1}^n x_i$  given the number of steps that occurred within  $\Delta t$ ,  $n$ .

The magnitude of the steps  $|x_i|$  is distributed exponentially with mean  $vk_{\text{off}}^{-1}$ , where  $v = F_0/\gamma$  is the particle

velocity due to one motor force. Since the sign of  $x_i$  is  $\pm 1$  with probability  $1/2$ ,  $x_i$  are i.i.d Laplace distributed with the probability density function (PDF)

$$f(x_i) = \frac{1}{2s} e^{-|x_i|/s}, \text{ for } s = vk_{\text{off}}^{-1}.$$

Thus the PDF of the sum of  $n$  such independent random variables  $\Delta x = \sum_{i=1}^n x_i$  is [1]:

$$P(\Delta x|n) = \frac{e^{-|\Delta x|/s}}{s(n-1)!2^n} \sum_{j=0}^{n-1} \frac{(n-1+j)!}{(n-1-j)!j!} \frac{(|\Delta x|/s)^{n-1-j}}{2^j} \quad (S3)$$

This is an exponential multiplied by a polynomial, as a function of  $\Delta x$ . Therefore it has an exponentially decaying tail. It is now left to show that  $P_n(n)$  decays fast enough that  $P(\Delta x(\Delta t))$  also has an exponentially decaying tail: it satisfies  $\lim_{\Delta x \rightarrow \infty} \frac{\log P(\Delta x)}{\Delta x} = c$  for a constant  $c < 0$ .

By substituting Eq. S3 into Eq. S2, rearranging the summations and shifting indices, we obtain:

$$P(\Delta x) = \frac{e^{-|\Delta x|/s}}{s} \frac{1}{2} \sum_{m=0}^{\infty} \frac{1}{m!} \frac{1}{2^m} f(m) \left( \frac{|\Delta x|}{s} \right)^m, \quad (S4)$$

where

$$f(m) = \sum_{j=0}^{\infty} P_n(j+m+1) \frac{(2j+m)!}{j!(j+m)!} \frac{1}{2^{2j}} \quad (S5)$$

Since  $P(\Delta x)$  is equal to  $e^{-|\Delta x|/s}$  times a series in  $|\Delta x|/s$  with positive coefficients, which hence diverges as  $|\Delta x| \rightarrow \infty$ , then  $P(\Delta x) > e^{-|\Delta x|/s}$  for a large enough  $n$ . If a constant  $C$  exists such that  $\forall m f(m) < C$ , then from Eq. S4 we conclude that  $P(\Delta x) < \frac{C}{2s} \exp(-|\Delta x|/2s)$ . Hence overall, for a large enough  $\Delta x$ ,  $P(\Delta x) \propto e^{-\beta|\Delta x|/s}$ , where  $1/2 < \beta < 1$ .

We will show that this is true in the limit of  $p_{\text{on}} \ll 1$ , where the number of steps  $n$  taken within  $\Delta t$  is Poisson distributed with mean  $\lambda \equiv k_{\text{on}}\Delta t$ :  $P_n(n) = e^{-\lambda} \lambda^n / n!$ . In this case:

$$f(m) = e^{-\lambda} \sum_{j=0}^{\infty} \frac{(2j+m)!}{j!(j+m)!(j+m+1)!} \frac{\lambda^{j+m+1}}{2^{2j}} \quad (S6)$$

This series converges for every  $m$ .

Define

$$g(m) = \frac{(2j+m)! \lambda^m}{j!(j+m)!(j+m+1)!} \quad (\text{S7})$$

then

$$\frac{g(m)}{g(m+1)} = \frac{j+m+2}{\lambda} \left( 1 - \frac{j}{2N+m+1} \right) > \frac{j+m+2}{2\lambda} \quad (\text{S8})$$

and therefore for  $m > 2\lambda - 2$ , regardless of  $j$ ,  $g(m)$  is a decreasing function. Therefore for such  $m$ ,  $f(m)$  is also a decreasing function. Thus  $f(m)$  has a maximal value for some  $M$  such that  $0 \geq M \geq 2\lambda - 2$ , and hence  $\forall m f(m) < f(M) \equiv C$ .

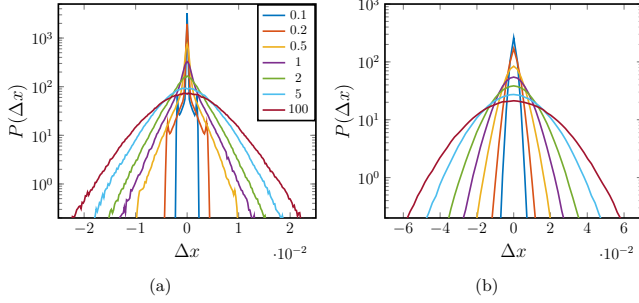

FIG. S1. Exponential tails in the weak confinement  $k/\gamma \ll k_{\text{off}}, k_{\text{on}}$  and small  $p_{\text{on}}$  limits. The van Hove distribution is plotted for varying lag times  $\Delta t$ , for  $k = 10$ ,  $\gamma = 50$ ,  $k_{\text{on}} = 1$ ,  $k_{\text{off}} = 10$  (a)  $N = 1$  (b)  $N = 10$ .

In numerical simulations of our model in the weak confinement regime  $k/\gamma \ll k_{\text{off}}, k_{\text{on}}$ , with a small but nonzero  $k$ , the van Hove distribution indeed displays exponential tails (Fig. S1). At short enough time scales, for small motor number  $N$  the van Hove distribution has peaks resulting from sampling of motion at nearly constant velocity during the entire sample time. Then, as  $\Delta t$  grows, exponential tails become evident until finally, at long enough times, the distribution is Gaussian nearly throughout the sampled domain of  $\Delta x$  values.

## 2. THE FAST PARTICLE LIMIT

The overdamped Langevin equation governing the motion of the particle in the limit where the friction coefficient  $\gamma$  is larger than all other rates in the system:

$$\gamma \dot{x} = -kx - \sum_{i=1}^N M_i F_0 \quad (\text{S9})$$

The solution of this equation for a given constant  $\sum_{i=1}^N M_i = N_{+1} - N_{-1} \equiv \Delta N$  is  $x(t) = (x(0) - \Delta N F_0/k) \exp(-k/\gamma t) + \Delta N F_0/k$ . Thus the typical timescale it takes the particle to reach the position corresponding to zero total force on it at a certain motor state is  $\gamma/k$ . Thus when  $k_{\text{off}}^{-1}, k_{\text{on}}^{-1} \gg \gamma/k$  the particle

moves between the peaks of  $P(x)$  much faster than the motor state changes, and therefore it spends much more time in the zero force positions of the motor states than moving between them. We will hence refer to this limit as the fast particle limit. It is also the limit of strong confinement, since the bulk elasticity  $k$  is large in this limit.

## 3. $P(x)$ AND THE LONG-TIME VAN HOVE DISTRIBUTION IN THE FAST PARTICLE LIMIT

In this section, we work in the fast particle limit  $\gamma k_{\text{off, on}}/k \ll 1$ , where the particle moves quickly between the peaks of the steady state distribution  $P(x)$ , which occur at positions where the motor force is balanced by the harmonic potential force. We use an approximation where we completely neglect the transition time between the peaks, and thus identify each motor state with a unique position of the particle in space.

Each  $N$  motor state  $\mathbf{M} = (M_1, M_2, \dots, M_N) \in \{0, \pm 1\}^N$  corresponds to a position  $x = x_0 \sum_{i=1}^N M_i$ , with  $x_0 = F_0/k$ , which the particle will reach in that motor state given enough time. We assume (as is approximately correct in the fast particle limit) that once the motor state changes, the particle immediately moves to its corresponding force balance position. Under this assumption each of the  $2N + 1$  peaks of the steady state particle position distribution are delta functions. Denote the probability of finding the particle in  $m x_0$  by  $P_m$ . Denote by  $N_{0, \pm 1}$  the number of  $M_i$  variables equal to  $0, \pm 1$  (the total number of motors is  $N_{-1} + N_0 + N_{+1} = N$ ). Denote the steady state ratio of time in which a single motor is on  $p_{\text{on}} = k_{\text{on}}/(k_{\text{on}} + k_{\text{off}})$ . Each time a motor turns on it randomly chooses a direction of  $\pm 1$ , so the probability to find a motor in the  $\pm 1$  state is  $\frac{1}{2} p_{\text{on}}$ . The probability to find a single motor in the off state is  $p_{\text{off}} = 1 - p_{\text{on}}$ . Thus the steady state distribution of  $(N_{+1}, N_{-1})$  is a trinomial distribution:

$$P(N_{+1}, N_{-1}) = \frac{N!}{N_{+1}! N_{-1}! (N - N_{+1} - N_{-1})!} \times \left( \frac{1}{2} p_{\text{on}} \right)^{N_{+1} + N_{-1}} p_{\text{off}}^{N - N_{+1} - N_{-1}} \quad (\text{S10})$$

Therefore the peaks of  $P(x)$  are given by:

$$P_j = P \left( \sum_{i=1}^N M_i = |j| \right) = \sum_{k=|j|}^N P(N_{+1} = k, N_{-1} = k - |j|) \quad (\text{S11})$$

In the long time limit, the van Hove distribution is equal to the convolution of the steady state position distribution with itself:  $P(\Delta x(\Delta t \rightarrow \infty)) = P(x) * P(x)$ . It has  $4N + 1$  peaks, which we will denote  $\tilde{P}_i$  for integer  $-2N \leq i \leq 2N$ , corresponding to particle positions  $x = i x_0$ . They are given by the discrete convolution

$$\tilde{P}_i = \sum_{j=-N}^N P_j P_{i-j} \quad (\text{S12})$$

where the  $P_j$  are given by Eq. S11 for  $-N \leq j \leq N$  and zero otherwise. We will now show that the long-time van Hove distribution for a system with  $N$  motors is equal to the steady state position distribution for a system with  $2N$  motors, i.e.  $\tilde{P}_i(N) = P_i(2N)$ . Proof:

$$\begin{aligned} P_i(2N) &= P \left( \sum_{k=1}^{2N} M_k = i \right) \\ &\stackrel{(*)}{=} \sum_{j=-N}^N P \left( \sum_{k=1}^N M_k = j \right) P \left( \sum_{k=N+1}^{2N} M_k = i - j \right) \\ &= \sum_{j=-N}^N P_j P_{i-j} = \tilde{P}_i(N) \end{aligned} \quad (\text{S13})$$

where the equality  $(*)$  is due to the independence of the motor state variables  $M_i$ . Therefore

$$\begin{aligned} \tilde{P}_j(N) &= P_j(2N) \\ &= \sum_{k=|j|}^{2N} \frac{(2N)!}{k!(k-|j|)!(2N-2k+|j|)!} \left(\frac{1}{2}p_{\text{on}}\right)^{2k-|j|} p_{\text{off}}^{2N-2k+|j|} \\ &= \frac{(2N)!}{|j|!(2N-|j|)!} \left(\frac{1}{2}p_{\text{on}}\right)^{|j|} p_{\text{off}}^{2N-|j|} + O(p_{\text{on}}^{|j|+2}) \end{aligned} \quad (\text{S14})$$

Thus to leading order in small  $p_{\text{on}}$ , the distance between consecutive peaks of  $P(\Delta x(\Delta t \rightarrow \infty))$  in log scale is:

$$\begin{aligned} \Delta_j &\equiv \log \left( \frac{\tilde{P}_j}{\tilde{P}_{j+1}} \right) \\ &\approx \log \left( \frac{p_{\text{off}}}{p_{\text{on}}} \right) + \log \left( \frac{j+1}{2N-j} \right) \end{aligned} \quad (\text{S15})$$

For  $p_{\text{on}} \rightarrow 0$ ,  $\Delta_j \approx -\log(p_{\text{on}})$ . Therefore in this limit the ratio of consecutive peak height differences  $r_j \equiv \frac{\Delta_j}{\Delta_{j+1}} \rightarrow 1$ . A plot of  $r_j$ , calculated using Eq. S14 (Fig. S2), reveals a stronger result:  $r_j < 1$  for all  $p_{\text{on}} < p_{\text{on}}^c$  for a rather large  $p_{\text{on}}^c$ . Thus  $p_{\text{on}}$  needs to be larger than  $p_{\text{on}}^c$  in order to obtain a  $r_j > 1$ .

#### 4. ONE SUSCEPTIBLE MOTOR IN THE FAST PARTICLE LIMIT

Consider a system with one motor ( $N = 1$ ) in the fast particle limit  $\gamma k_{\text{off, on}}/k \ll 1$ . In this case, the steady state particle density has three peaks at 0 and  $\pm x_0$ , for  $x_0 = F_0/k$ . In this limit the particle spends a small

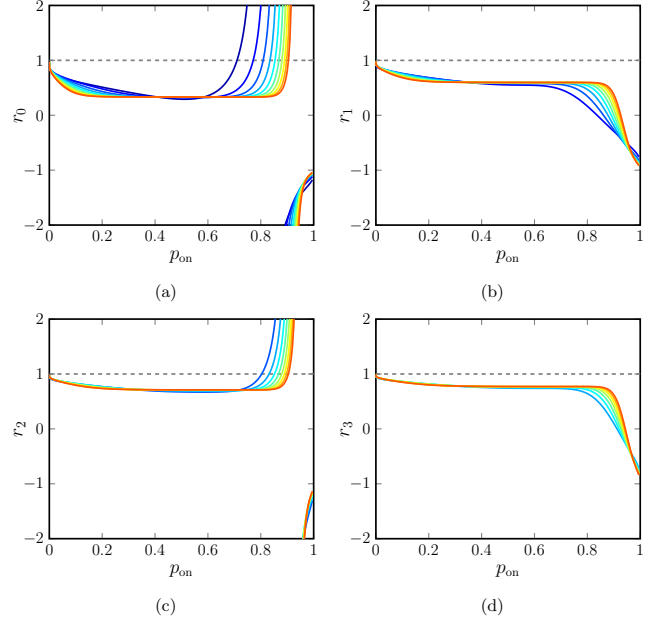

FIG. S2. (a-d) The results of the theoretical calculation of the long-time van Hove peak ratio  $r_i$  for  $i = 0 - 3$  in the fast particle limit. Plots are for motor number  $N = 1 - 10$  where the line color denotes the motor number and varies between dark blue ( $N = 1$ ) and red ( $N = 10$ ). Note  $r_i \rightarrow 1$  as  $p_{\text{on}} \rightarrow 0$ , and  $r_i < 1$  for  $p_{\text{on}} \lesssim 0.6$  for all shown parameters.

amount of time at positions that are not  $x = 0, \pm x_0$ . Thus we neglect all other states and treat the system as if it has 3 possible states, defined by the motor states  $M = 0, \pm 1$ , which correspond to a unique particle position  $x = 0, \pm x_0$ . We generally assume that the rate of transition between two states can depend on the current  $x$  and the nonzero  $M$  state involved (which could be the  $M$  value associated with the state from or into which the transition occurs), and denote the rates of transitions between these states:

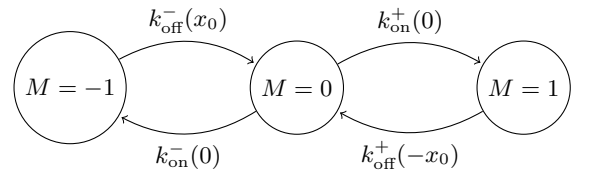

Assume that the rates depend only on  $MF_{\text{elastic}} = -Mkx$ . Thus the system is symmetric to reflection of  $x \rightarrow -x$   $M \rightarrow -M$ . Therefore  $k_{\text{on}}^-(0) = k_{\text{on}}^+(0) \equiv k_{\text{on}}(0)/2$ , and  $k_{\text{off}}^+(x_0) = k_{\text{off}}^-(x_0) \equiv k_{\text{off}}(\pm x_0)$ .

The master equations for the system:

$$\begin{aligned} \partial_t P(-x_0) &= \frac{k_{\text{on}}(0)}{2} P(0) - k_{\text{off}}(-x_0) P(-x_0) \\ \partial_t P(x_0) &= \frac{k_{\text{on}}(0)}{2} P(0) - k_{\text{off}}(x_0) P(x_0) \\ \partial_t P(0) &= -k_{\text{on}}(0) P(0) + k_{\text{off}}(-x_0) P(-x_0) + k_{\text{off}}(x_0) P(x_0) \end{aligned} \quad (\text{S16})$$

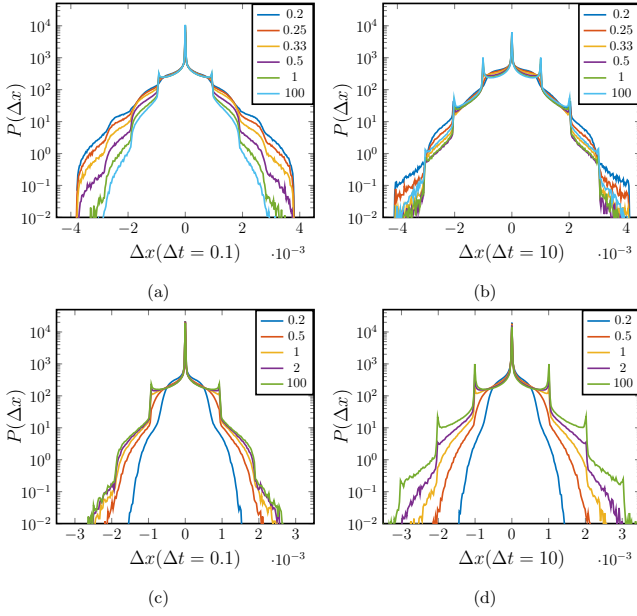

FIG. S3. Comparison of systems of  $N = 2$  susceptible motor with susceptibility in the on or off rate. The van Hove distribution for various  $F_1$  values is plotted for: (a-b)  $k_{\text{on}}^{\pm} = k_{\text{on}}^0 e^{\pm kx/F_1}$ ,  $k_{\text{off}} = 10$ , for lag times of  $\Delta t = 0.1$  (a) and  $\Delta t = 10$  (b). Visibly, for the short lag time  $\Delta t = 0.1$  increasing the susceptibility (decreasing  $F_1$ ) increases the height of the shoulder  $\tilde{P}_2$  and therefore increases  $r_0$ . (c-d)  $k_{\text{on}} = 1$ ,  $k_{\text{off}} = 10e^{-Mkx/F_1}$ , for lag times of  $\Delta t = 0.1$  (c) and  $\Delta t = 10$  (d). Increasing the susceptibility causes peaks to become shoulders and move to smaller  $|x|$ . It does not increase  $\tilde{P}_2$  or  $r_0$ . ( $k = 1000$ ,  $F_0 = 1$ ,  $\gamma = 50$ )

The steady state solution of the master equations S16 is thus:  $P(x_0) = P(-x_0) = \frac{k_{\text{on}}(0)}{2k_{\text{off}}(x_0)} P(0)$ .

Note that the dimensionless ratio  $k_{\text{on}}(0)/k_{\text{off}}(x_0)$  controls the steady state distribution. Therefore, if  $k_{\text{off}}$  is  $x$  dependent, the steady state distribution will vary as the susceptibility of the motor is increased since  $k_{\text{off}}(x_0)$  will vary. On the other hand, if  $k_{\text{off}}$  is constant but  $k_{\text{on}}$  varies in space, since at  $x = 0$  there is not external force, increasing the susceptibility of the motor will not change the steady state particle position distribution.

## 5. THE VAN HOVE DISTRIBUTION FOR $N = 2$

We show that the results discussed and showed in the main text about the van Hove peak and shoulder structure for  $N=1$ , hold also for  $N=2$ , by plotting the  $N=2$  equivalents of Fig. 3 and Fig. 4. Namely,  $r_0 > 1$  is obtained for a susceptible  $k_{\text{on}}$  at a small enough lag time  $\Delta t$ , while for a susceptible  $k_{\text{off}}$ ,  $r_0$  does not become substantially greater than 1 for all lag times.

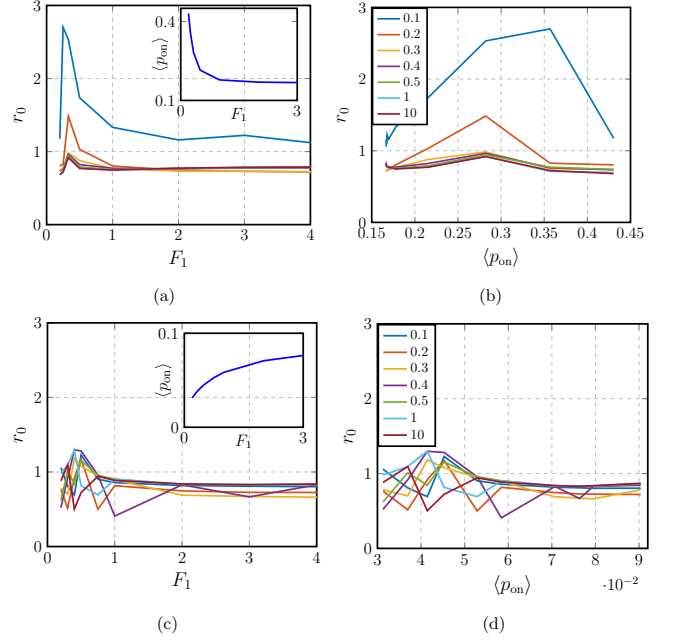

FIG. S4. The effect of susceptibility of the active event occurrence rate  $k_{\text{on}}$ . For the model with  $k_{\text{on}}^{\pm} = e^{\mp kx/F_1}$ ,  $k_{\text{off}} = 10$ ,  $N = 2$ : (a)  $r_0$  as a function of  $F_1$  for various lag times  $\Delta t$ . Inset: The average time ratio in which the motor was on  $\langle p_{\text{on}} \rangle$  as a function of  $F_1$ . (b)  $r_0$  as a function of the average duty cycle  $\langle p_{\text{on}} \rangle(F_1)$  for various lag times  $\Delta t$ . Note that for a small enough  $\Delta t$ ,  $r_0 > 1$  for much smaller  $p_{\text{on}}$  than in the adamant motor system. (c,d) Same as (a) and (b) for  $k_{\text{on}} = 1$ ,  $k_{\text{off}} = 10e^{-Mkx/F_1}$  ( $k = 1000$ ,  $F_0 = 1$ ,  $\gamma = 50$ )

## 6. SIMULATION DETAILS

We performed simulations in which the Langevin equation of motion Eq. 1 was integrated using the Euler method.

The particle steady state position distribution and the van Hove displacement distribution for various lag times were estimated from the results, by calculating a normalized histogram. Peaks and shoulders were automatically detected, using algorithms that rely on the mathematical definition of peaks and shoulders but also using known features of the distributions our model produces in order to avoid false positives due to noise. Example results of the detection algorithm are plotted in Fig. 1d.

Additional details about the simulation results presented in figures: The results presented for each parameter set are from simulations with the following properties:

Fig. 1c,d, 2: time difference between samples of the particle position: 0.05, total simulation run time:  $10^6$ .

Fig. 3,4a,b: time difference between samples of the particle position: 0.1, total simulation run time:  $2 \times 10^5$ .

Fig. 4c,d: time difference between samples of the particle position: 0.1, total simulation run time:  $3 \times 10^6$ .

Fig. S1: time difference between samples of the particle position: 0.1, total simulation run time:  $10^5$ .

Fig. S3,4: time difference between samples of the particle position: 0.1, a,b: total simulation run time:  $2 \times 10^6$ ,

c,d:  $5 \times 10^6$ .

The simulation step size was  $10^{-4}$  in all of the simulations.

---

[1] S. Kotz, T. Kozubowski, and K. Podgorski, *The Laplace distribution and generalizations: a revisit with applications*

*to communications, economics, engineering, and finance* (Springer Science & Business Media, 2012).
